# Supplementary material for: The ferroelectric domain wall phonon polarizer
Source: arXiv:1710.00663 source file (2017-10-02)
Supplement: Supplementary file 1 [file Supplemal_material_v_resubmit.pdf]

# Supplemental Material for "A phonon polarizer based on ferroelectric domain walls"

Miquel Royo,[1] Carlos Escorihuela-Sayalero,[2] Jorge Íñiguez,[2] and Riccardo Rurali[1]

[1]*Institut de Ciència de Materials de Barcelona (ICMAB–CSIC) Campus de Bellaterra, 08193 Bellaterra, Barcelona, Spain*

[2]*Materials Research and Technology Department, Luxembourg Institute of Science and Technology, 41 rue du Brill, L-4422 Belvaux, Luxembourg*

## SUPPLEMENTAL METHODS

### Computational details

The key magnitude to initialize any NEGF transport simulation is the surface Green's function of the semi-infinite contacts ($\mathbf{g}^r_{L/R}(\mathbf{k}_\perp,\omega)$). This function needs only to be computed for those atomic positions in the contacts located near the channel and forming what is known as principal or surface layer, i.e., those atoms with effective interaction with any atom in the channel. We calculate $\mathbf{g}^r_{L/R}(\mathbf{k}_\perp,\omega)$ following an efficient iterative approach [1]. Then we access the single mode transmission analysis by means of the contacts Bloch matrices, which can be computed from the surface Green's functions as detailed in Ref. 2. On the one hand, we extract the frequency, longitudinal wave vector ($k$) and polarization of the extended phonons at both contacts from the eigenvalues and eigenvectors of the Bloch matrices. On the other hand, we calculate a transmission matrix $\mathbf{t}$ whose elements give the probability of transmission between the phonon modes at both contacts across the channel. Thus, we can associate a transmission probability between 0 and 1 to each phonon mode in the left or the right contact at a given ($\mathbf{k}_\perp$,$k$,$\omega$) point. The total transmission function $\mathcal{T}(\omega)$, as obtained in conventional NEGF methods, is calculated through summation of the contributions from all phonon modes in one of the two contacts (the outcome is symmetric) and integration over the transverse wave vector. Finally, we calculate the thermal conductance due to ballistic transport of phonons, i.e., neglecting the anharmonic phonon-phonon scattering in the transport process, with the well-known linear response Landauer formalism.

To obtain the force-constant matrix elements necessary for the the NEGF transport simulations we use the second-principles model potentials developed by one of us and introduced in Ref. 3. We perform a structural relaxation of a supercell that comprises both contacts and channel atomic positions by means of a Monte Carlo simulated annealing in which the temperature is reduced up to essentially zero Kelvin. In order to enforce a given metastable multidomain configuration we initialize the relaxation with a supercell in which abrupt domain interfaces are artificially introduced. The force-constant matrix elements are later calculated by the small-displacement method, i.e., displacing once at a time all the atoms of the supercell along the three Cartesian components and evaluating the ensuing forces. Periodic boundary conditions are assumed all the way.

Unless otherwise stated we employ a supercell for the simulations with a transverse cross section of $4 \times 4$ primitive cells. This enables the evaluation of the thermal transport at 25 commensurate $\mathbf{k}_\perp$ points generated with a Monkhorst-Pack scheme ensuing convergence of both phonon transmission and thermal conductance. More critical is the choice of the number of primitive cells along the longitudinal (transport) direction. Taking the case of a monodomain system as a test bed, we have observed that in order to recover an integer phonon transmission function at small values of $\mathbf{k}_\perp$, the channel and the contacts principal layer need to be of the same length. The question, grounded on the slow decay of the long-range dipole-dipole interactions in insulating materials, is carefully analyzed below. Therefore, in all the calculations here presented we use the same number of primitive cells along the longitudinal direction in both channel and contacts principal layer.

**Reliability of the computational scheme**

Considering as benchmark calculations (free of any parameterization) *ab initio* density functional theory (DFT) calculations, the technique of SPMP represents a simplified alternative that allow us dealing with large-scale multidomain ferroelectric systems that could not be handled at the DFT level. The method is based on the calibration of a set of potential parameters to reproduce DFT results and is specifically realized for each material under study. A detailed description of the procedure followed to calibrate the model potential for $PbTiO_3$ employed in the manuscript calculations was presented in Ref.3. There one can see how the phonon band dispersions (and therefore the second order force-constants) obtained with the model potential, correctly reproduce those from DFT calculations. Further, in Ref.4 the $PbTiO_3$ model potential is demonstrated to almost perfectly reproduce the atomic distortions occurring at 180° domain walls obtained with DFT (see, e.g., local polarizations in Figure 1 in Ref.4). Note that a correct relaxed atomic structure and second-order force constants are the only information that we extract from the SPMP calculations in order to evaluate the phonon transport properties. Therefore, given that in both cases our model reproduces DFT results almost exactly, we are confident that the main result of our manuscript, i.e., the longitudinal phonon polarizer effect, would be validated by a parameter-free DFT calculation in case such a formidable calculation was computationally tractable.

Regarding the NEGF phonon transport calculations, these are free from any parameterization and the convergence of the calculations against system dimensions in real and reciprocal space has been checked as detailed in Section . As regards our NEGF calculations, the only approximation we assumed was to neglect electron-phonon and phonon-phonon interactions, whose inclusion in the NEGF formalism is possible, but computationally realizable only in the simplest (smallest) of systems. We believe that such an approximation does not affect the main result of our paper for the following reasons. First, electron-phonon interactions are known to be only relevant in metals or doped semiconductors, whereas here we focus on an insulating material (ferroelectrics tend to be good insulators, so this aspect is not specific to $PbTiO_3$). Second, at low temperatures, with only low-frequency and low-momentum phonon modes excited, phonon-phonon interactions are negligible in good approximation. Further, we have very recently studied the interface thermal boundary resistance of a 180° domain wall in $PbTiO_3$ at 500 K with nonequilibrium molecular dynamics (NEMD), a methodology that accounts for all orders of anharmonicity in the phonon-phonon scattering, and obtained an excellent agreement with the value extracted from the NEGF calculations of the present manuscript [5]; interestingly, the fact that both NEGF and NEMD methodologies predict that the same amount of phonons are scattered at the DW strongly suggests that our predicted polarizer effect might remain active at high temperatures.

**Treatment of long-range interactions in NEGF calculations.**

The second-principles model potentials employed to describe the interatomic interaction include long-range dipole-dipole terms that conflict with the general NEGF approach. In particular, the calculation of the contacts surface Green's function assumes first-nearest-neighboring interaction between principal layers, which means that by delimiting the length of the principal layer we are artificially introducing a cut off distance in the long-range interactions. In principle, such conflict may be eluded by enlarging the size of the principal layers along the longitudinal transport direction. However, in insulating materials as the one studied here dipole-dipole interactions decay very slowly and we have observed that increasing the size of the principal layers does not completely cancel artifacts ensuing from this cut off.

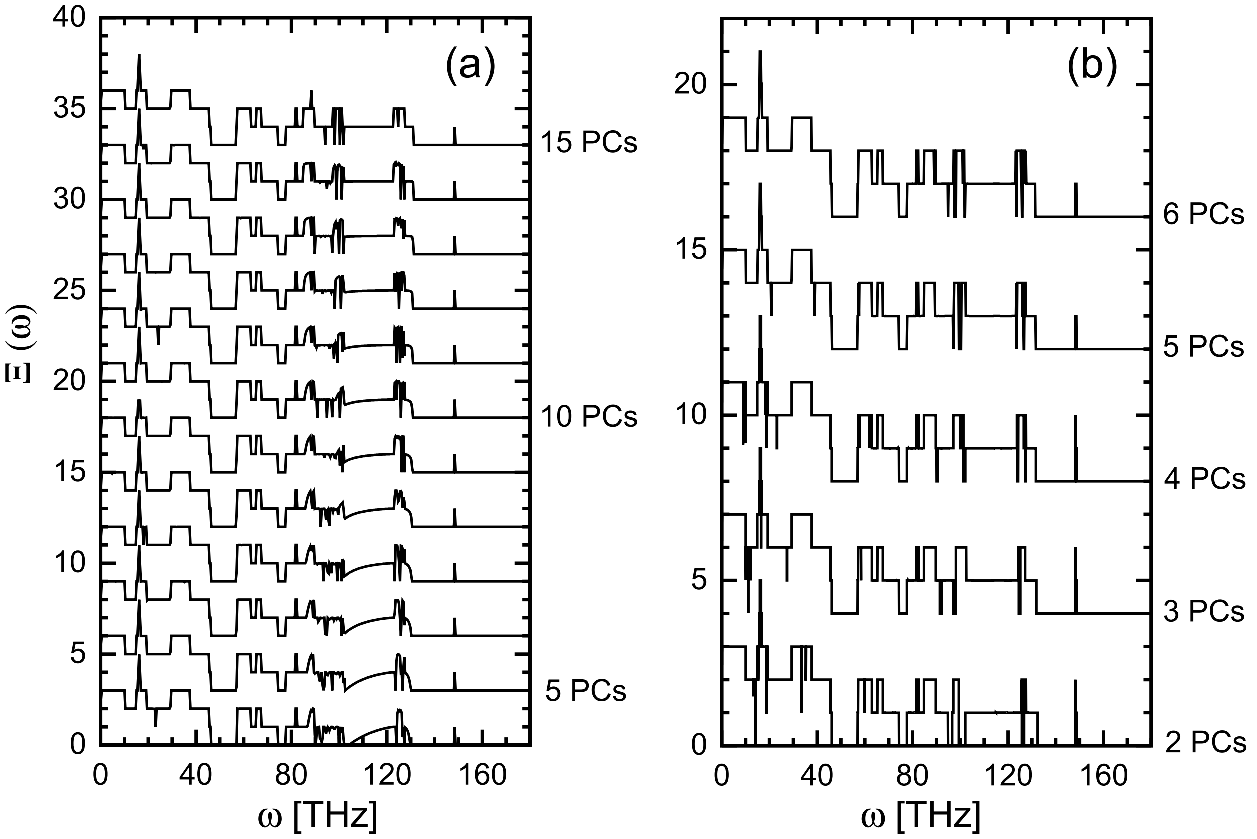


FIG. S1. Phonon transmission functions for a monodomain PTO sample calculated at $\mathbf{K}_{\perp}^{*} = 0$ using different lengths for channel and contact. In (a) a fixed channel length of 15 primitive cells (PCs) has been assumed and the number of cells in the contacts is increased from 4 PCs (bottom line) to 15 PCs (top line) as indicated. In (b) the same number of PCs are used in channel and contact. Consecutive transmission curves are split for clarity.

The main artefact we observe is the appearance of unphysical noninteger phonon transmissions for homogeneous (monodomain) $PbTiO_3$. This effect can be observed in Fig. S1 (a) that shows transmissions calculated at $\mathbf{K}_{\perp}^{*} = 0$ for a system with 15 primitive cells (PCs) in the channel and different number of PCs in the contacts. The transmission function correctly acquires integer values, denoting the number of phonon modes accessible at a given frequency, up to $\omega \sim 80$ THz. However, for frequencies between 85 and 130 THz an anomalous region with noninteger transmissions shows up. This unphysical result gets gradually corrected as more PCs are included in the contact principal layer but it only completely disappears when the same number of PCs is used to define the channel and the contact. Noticeably, noninteger transmissions also reappear if the contact includes more PCs than

the channel (not shown).

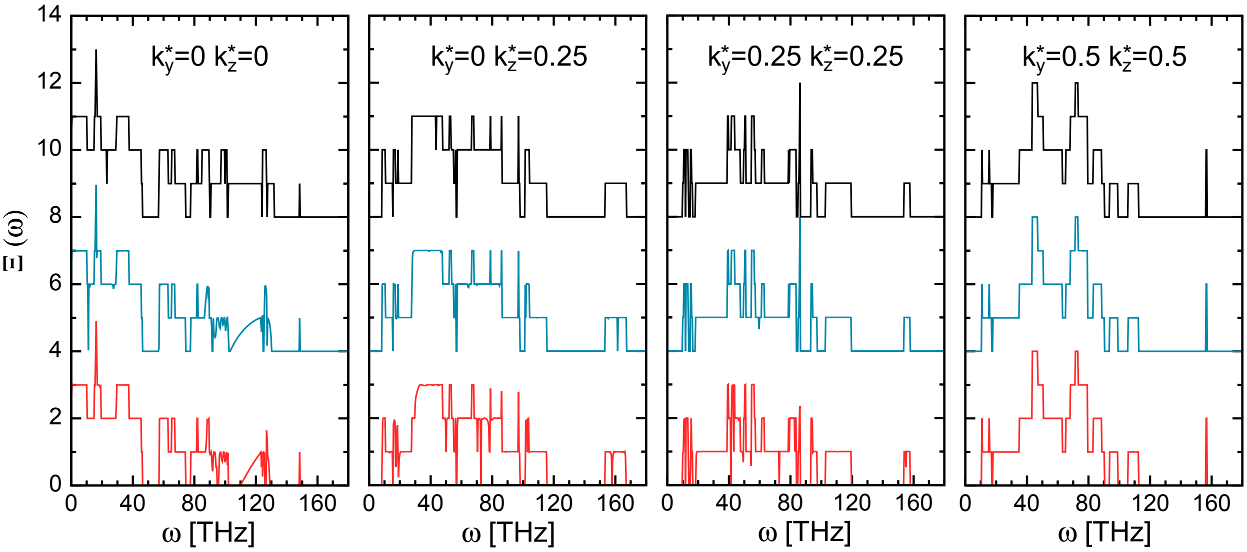


FIG. S2. Phonon transmission function for a monodomain PTO channel of length of 4 primitive cells (PCs) calculated employing different number of PCs to define the contacts: 2 PCs (red lines), 3 PCs (blue lines) and 4 PCs (black lines), transmission curves are split for clarity. Results are shown for four different reduced transverse wave vectors, $\mathbf{K}_\perp^* = (k_y^*, k_z^*)$, as indicated.

Therefore, in order to avoid unphysical transmissions one needs to have contacts and channel of the same length. This is because, otherwise, the cut off introduced on the long-range interactions is different to the left and right directions from the contact. Due to this asymmetry the atoms in the contact surface layer interact in a different manner with the atoms of the channel and those in the next principal layer deeply placed in the contact. For this reason the system is interpreted by the method as nonhomogeneous, and noninteger transmissions occur. Fig. S1 (b) shows that the problem disappears by using the same length for contacts and channel and that the transmissions computed in this way show a fast convergence with the total length.

Besides, it must be noted that such noninteger transmissions for the homogeneous system are only observed for small values of the transverse wave vector $\mathbf{K}_\perp^*$, i.e., for transmissions associated with phonons traveling neatly parallel to the longitudinal direction. Fig. S2 shows how at finite values of $\mathbf{K}_\perp^*$ the effect is considerably reduced and it even disappears despite using a small number of PCs to describe the contacts. Hence, although in our calculations we have properly used the same length for contacts and channel, it is to be expected that

the main results will not be greatly affected by this choice.

## SUPPLEMENTAL RESULTS

### Domain wall spacing effect on the phonon transport

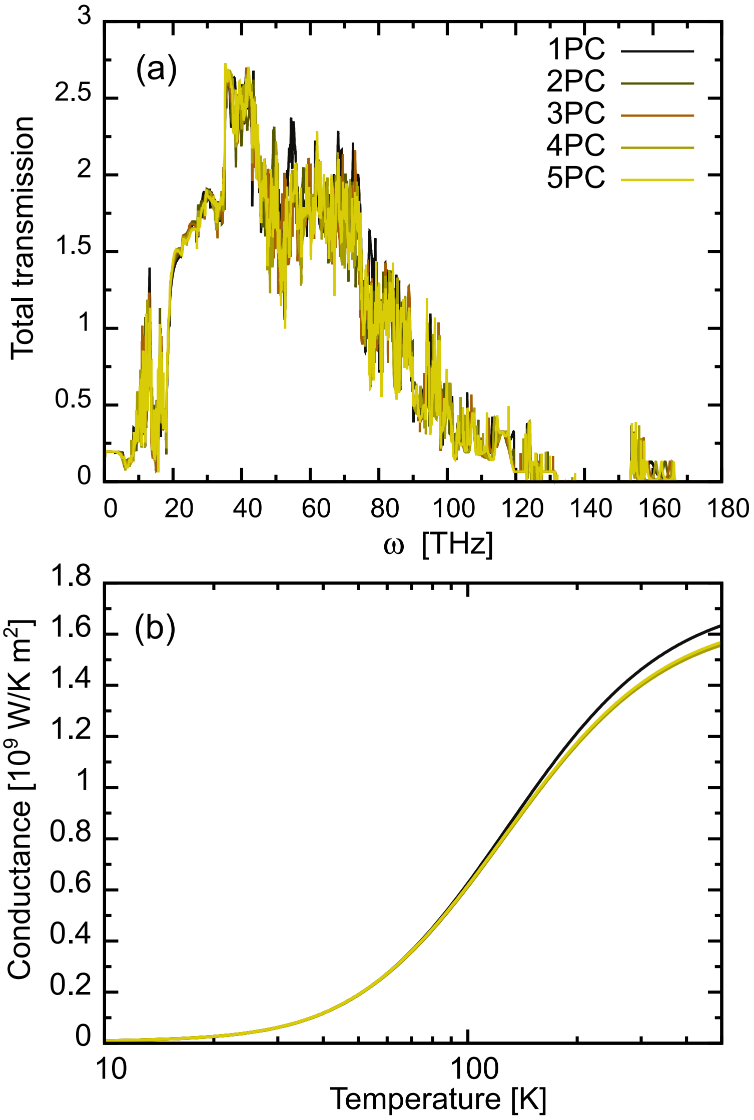


FIG. S3. (a) Total phonon transmission function and (b) thermal conductance calculated for PTO samples with 2 DWs spatially separated by different number of primitive cells (PCs) as indicated. It is observed that DW spacing has a negligible effect on the phonon transport, except for the extreme case in which a single PC separates the two DWs.

### Polarization resolved thermal conductance

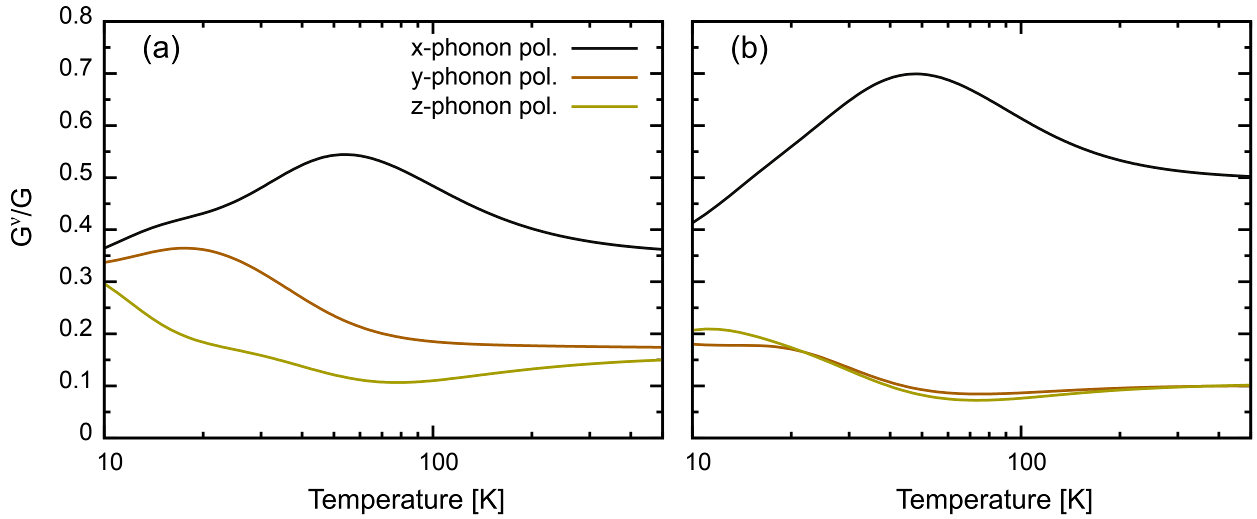


FIG. S4. Fraction of thermal conductance for a monodomain (a) and a 1DW (b) PTO sample due to phonons at least 70% polarized along $\nu = x$, $y$ and $z$ directions. Thermal transport is calculated along $x$ and the ferroelectric polarization is parallel to $z$. The DW in (b) reduces the conductance by likewise scattering phonons polarized along $y$ and $z$.

### Phonon transport through curved domain walls

To probe the robustness of the longitudinal phonon polarizer effect against deviations of the ideally flat DW geometry we have performed thermal transport simulations in samples with DWs displaying certain curvature out of the $x, y$ plane. The studied geometries including one curved and one flat DWs, and two curved DWs are respectively shown in Figs. S5 (c) and (d). In these calculations we have not performed a Fourier transform over the transverse directions since the larger periodicity motif, which now involves up to 5x5 primitive cells in order to define de DW curvature, requires huge supercells that cannot be computationally handled. Instead, we have carried out a single transport calculation through a channel of 5x5 primitive cells thickness in the transverse direction. Strictly speaking, we have simulated the heat transport by exclusively taking into consideration the contribution from the transverse $\Gamma$-point. We note, thought, that the structural relaxation and force-constants calculation have been performed assuming periodic boundary conditions in all three directions.

Fig. S5 (a) compares the lattice thermal conductance for the two curved DWs geometries of panels (c) and (d), for a monodomain sample and a sample with 2 flat DWs. It is observed that the roughness introduced by the DW curvature leads to a more effective interfacial phonon scattering as the conductance reduction in curved DW samples (dashed lines) is more pronounced than for the counterpart sample with 2 flat DWs (brown solid line). On the other hand, in panel (b) we show the fraction of thermal conductance due to longitudinally polarized phonons. Noteworthy, data in this figure demonstrate that the longitudinal polarizer effect almost entirely survives the DW curvature for temperatures below 50 K, while at higher temperatures flat DWs are better polarizers than curved ones.

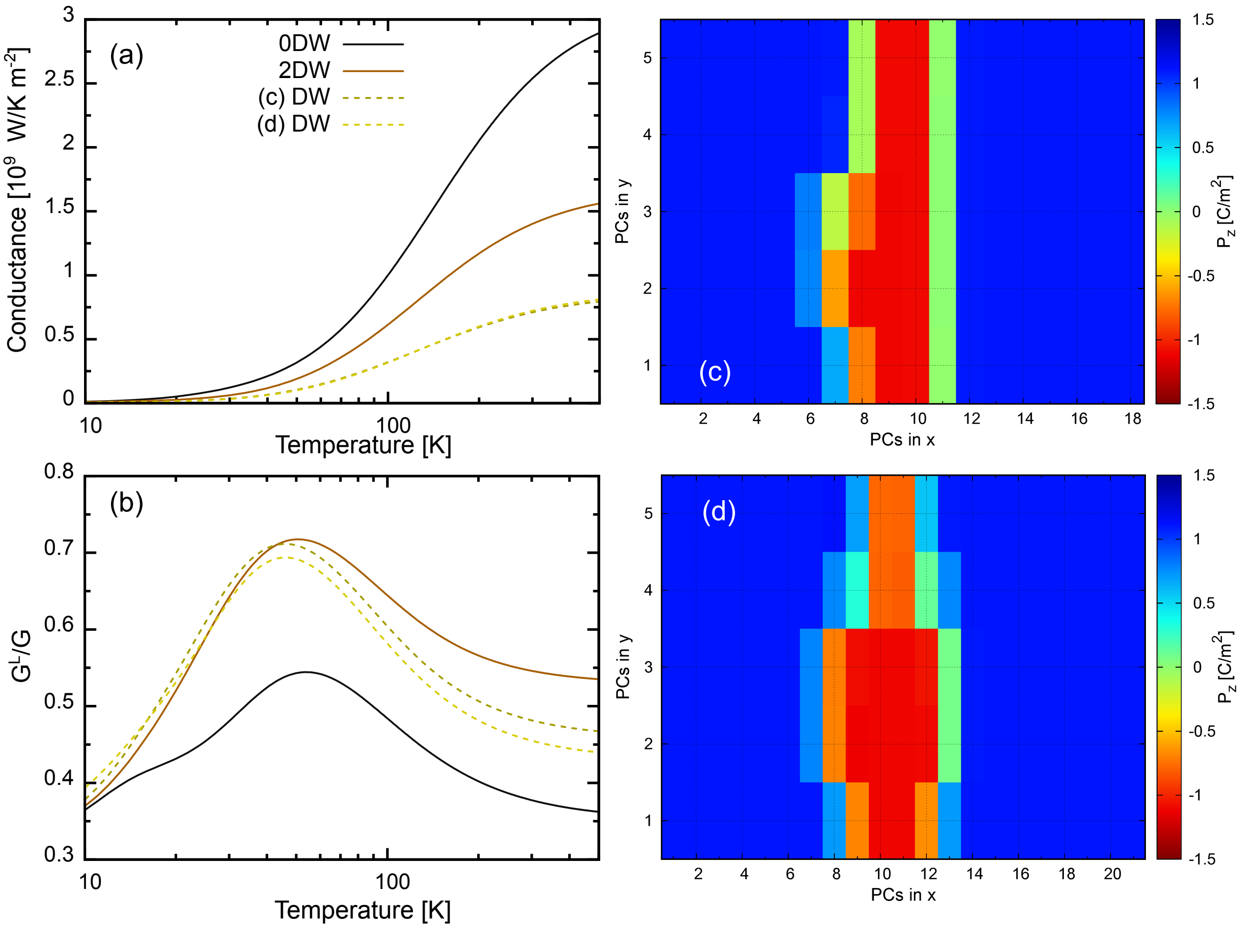


FIG. S5. Total thermal conductance for transport along the $x$-direction (a) and fraction of conductance due to phonons at least 70% longitudinally polarized (b) for two channels with curved DWs (dashed lines) whose ferroelectric polarization $P_z$ is represented over the $x, y$-plane in panels (c) and (e). The results for a monodomain sample and a sample with two flat 2 DWs in series are also shown for comparison (solid lines).

[1] M. P. L. Sancho, J. M. L. Sancho, and J. Rubio, J. Phys. F Met. Phys. **14**, 1205 (2000).

[2] Z. Y. Ong and G. Zhang, Phys. Rev. B **91**, 174302 (2015).

[3] J. C. Wojdeł, P. Hermet, M. P. Ljungberg, P. Ghosez, and J. Íñiguez, J. Phys. Condens. Matter **25**, 305401 (2013).

[4] J. C. Wojdeł and J. Íñiguez, Phys. Rev. Lett. **112**, 247603 (2014).

[5] J. Seijas-bellido, C. Escorihuela-salayero, M. Royo, P. Mathias, J. C. Wojdeł, J. Íñiguez, and R. Rurali, Submitted.
